# Supplementary material for: Denoising-based UNMT is more robust to word-order divergence than MASS-based UNMT
Source: arXiv:2303.01191 source file (2023-03-02)
Supplement: Supplementary file 1 [file appendixcolin.pdf]

# Appendix

May 2022

## 1 Preordering tool

The re-ordering tool we use is a rule-based system which re-order a sentence as shown in Figure 1.

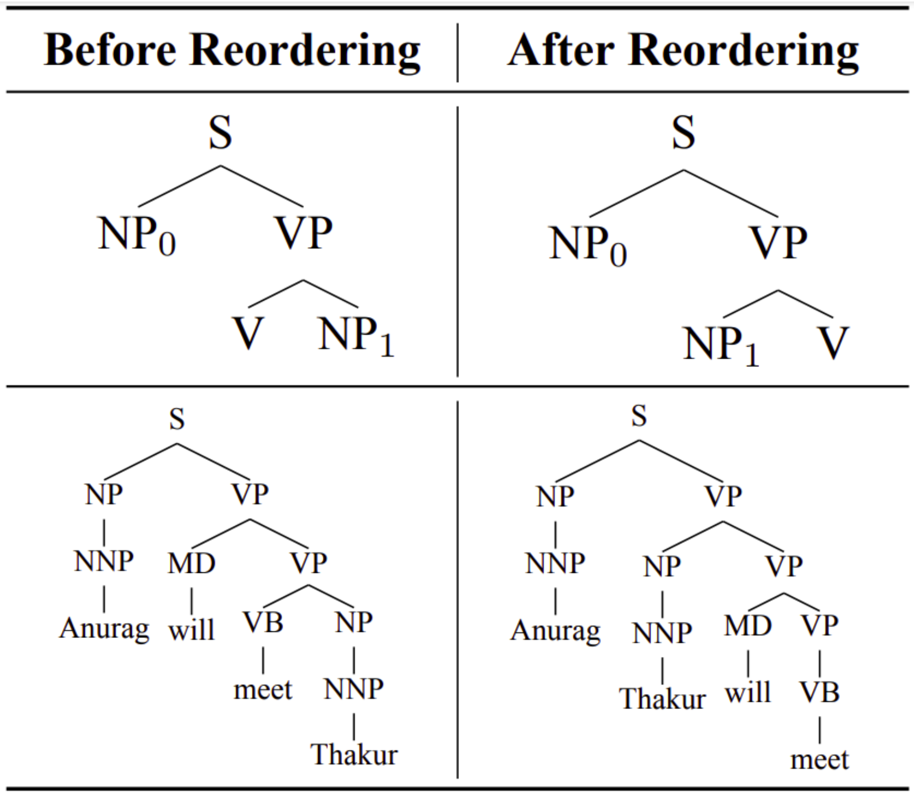


Figure 1: Example of reordering using the re-ordering tool we used (Chatterjee et al., 2014)

## 2 Handling re-ordering error

The tool we used generated parse error for some English sentences. In order to maintain equality, we removed those monolingual sentences or sentence-pairs from both original and re-ordered data. We perform all the experiments on the remaining data.

## 3 Demerit of training UNMT models with re-ordering

<table>
<tr><td>English source sentence</td><td>We need to change this mindset .</td></tr>
<tr><td>Reordered English source sentence</td><td>We this mindset change to need .</td></tr>
<tr><td>Hindi reference</td><td>हमें इस सोच को बदलने की ज़रूरत है ।<br>hameM isa socha ko badalane kI jarUrata hai |</td></tr>
<tr><td>Translation using DAE-static</td><td>हमें इस मानसिकता को बदलना होगा ।<br>hameM isa mAnasikatA ko badalanA hogA |<br>We need to change this mindset .</td></tr>
<tr><td>Translation using reordered-DAE-static</td><td>हम मानसिकता में बदलाव की जरूरत नहीं है ।<br>hama isa mAnasikatA meM badalAva kI jarUrata nahIM hai |<br>We don't need a change in mindset [case-marker is missing in output]</td></tr>
</table>

Figure 2: Translation example where re-ordering creates ambiguity

Hindi has three noun cases (nominative, oblique, and vocative) and five pronoun cases (nominative, accusative, dative, genitive, and oblique). Dative case-markers are often similar to accusative case-markers. There are only three cases in modern English, they are subjective, objective and possessive (his). After re-ordering it creates problem.

In the example shown in Figure 2, reference translation of the subject 'we' is 'hameM' which is in dative case. When we re-order the English sentence, it remains 'we' which is subjective case and whose frequent Hindi translation is 'hama'. In the translation produced by re-ordered model, we see the word 'hama' instead of 'hameM'.

## References

Rajen Chatterjee, Anoop Kunchukuttan, and Pushpak Bhattacharyya. 2014. Supertag based pre-ordering in machine translation. In *Proceedings of the 11th International Conference on Natural Language Processing*, pages 30–38.
